# Supplementary material for: FixEval: Execution-based Evaluation of Program Fixes for Programming Problems
Source: arXiv:2206.07796 source file (2023-03-30)
Supplement: Supplementary file 1 [file appendix.tex]

\section{Further Details of our Analysis}
\label{app:qual_examples}
\subsection{Description of Test Suite Collection}
\label{app:tests}
On the AtCoder website, we found the names of each contest.\footnote{\url{https://atcoder.jp/contests/}} Contests are named in the format of ABC123, AGC123, or ARC123 to indicate the AtCoder Beginner Contest, AtCoder Grand Contest, or AtCoder Regular Contest, followed by the specific contest number (i.e. 123 in this example) to create a unique identifier for a given problem. The name and contest number are also stored on CodeNet, where we get the exact same name and the contest number with problems sorted by difficulty. We then match these to retrieve the test cases in addition to input and expected output values from the DropBox link to create the test suite for \textbf{\textsc{FixEval}}. 
\section{Limitations}

% \textcolor{red}{Move to appendix?} 
There are a few limitations of the dataset presented in this work. In our experiments, we manually analyze the mistakes made by models with and without access to verdict information. We find that common model mistakes include additions of code segments that are unnecessary to fix a given bug. We believe this is due to insufficient information about the bug and the problem. Another limitation of this work is that, while the code bug fix pair dataset can be extended for other programming languages, code, and test suite expansion for more problems is solely dependent upon AtCoder availability. 
Also, the execution-based evaluation metric calculation requires a substantial amount of time to evaluate a single program. To reduce computation complexity, we select two data points randomly per problem from the test dataset. Nevertheless, parallelism and high-performance computing can be utilized towards making execution-based evaluation faster and more efficient for large-scale data.
In terms of research insights, our dataset incorporates Java and Python bugs, and may not generalize to other programming languages. Further research is necessary to evaluate the impact of FixEval for analyzing deep learning models for additional languages. Additionally, competitive programs submitted online may not accurately reflect real-world software bugs from professional developers. More work is necessary to develop benchmarks that simulate authentic software programs to evaluate deep learning models for automated program repair. %\il{In this work, we introduce \textsc{\textbf{FixEval}} as a useful context-aware dataset for evaluating models for bug fixing on programs with varying sizes and difficulties that incorporate space and time constraints.}\il{revise this and contribution \#1 , see the email, possible parsing variants with a different meaning. Does not seem to connect well with the last limitation. Should we skip this part? Or revise to better connect.}

%\todo{In general, need to organize this as: Limitation -> how we mitigate it/why it is necessary}

\subsection{List of Verdicts}
\label{app:verdicts}

The following is a list of all the possible verdict outcomes for submitted competitive programs with a brief description :

% \begin{itemize}
% \item Accepted (AC)
% \item Wrong Answer (WA)
% \item Compile Error (CE)
% \item Runtime Error (RE)
% \item Presentation Error (PE)
% \item Time Limit Exceeded (TLE)
% \item Memory Limit Exceeded (MLE)
% \item Output Limit Exceeded (OLE)
% \item Waiting for Judging (WJ)
% \item Waiting for Re-judging (WR)
% \item Judge Not Available (JNA)
% \item Internal Error (IE)
% \end{itemize}
% Not sure what's going on with the itemized list?

\textbullet~~\textbf{Accepted (AC):} Passed all test cases. \vspace{0.10cm} \\
\textbullet~~\textbf{Wrong Answer (WA):} Failed one or
more test cases.\vspace{0.10cm}  \\
\textbullet~~\textbf{Compile Error (CE):} Program did not compile.\vspace{0.10cm}  \\
\textbullet~~\textbf{Runtime Error (RE):} Program execution was not successful.\vspace{0.10cm}  \\
\textbullet~~\textbf{Presentation Error (PE):} Output is correct, but it is not formatted in the proper way.\vspace{0.10cm}  \\
\textbullet~~\textbf{Time Limit Exceeded (TLE):} The program did not run within the intended time limit.\vspace{0.10cm} \\
\textbullet~~\textbf{Memory Limit Exceeded (MLE):} The program did not run within the intended memory limit. \vspace{0.10cm} \\
\textbullet~~\textbf{Output Limit Exceeded (OLE):} Program tried to write too much information. \vspace{0.10cm} \\
\textbullet~~\textbf{Waiting for Judging (WJ):} Judge is busy. \vspace{0.10cm} \\
\textbullet~~\textbf{Waiting for Re-judging (WR):} Waiting for Judge to run the tests again. \vspace{0.10cm} \\
\textbullet~~\textbf{Judge Not Available (JNA):} Error encountered by Judge. \vspace{0.10cm} \\
\textbullet~~\textbf{Internal Error (IE):} Judge encountered an error or the problem setter's configuration is incorrect.

% \newpage
\input{figure/solved_with_verdict_mint}

% \subsection{Java Examples Solved only by the model with verdict in Figure \ref{fig:example_2}}

%\input{figure/solved_with_verdict}

% \newpage
% \subsection{Generated Python code examples with the CodeT5 model in Figure \ref{fig:example_2_python}}
\begin{figure*}[t]
\centering

\begin{tabular}{p{13.5cm}}
\toprule
Model learned to cast the output \\
\bottomrule
\end{tabular}

\vspace{5pt}
\begin{tabular}{l}
\begin{adjustbox}{valign=t,minipage=0.47\textwidth}
\begin{center}
    \underline{Buggy Program in Python}
\end{center}
\begin{tabular}{l}

\lstset{escapechar=~,style=CustomPy}
\begin{lstlisting}[ 
    linebackgroundcolor={%
    \ifnum\value{lstnumber}=2
        \color{red!10}
    \fi
    }
]
n = int(input())
n = print(int(n-1+1)*(n-1)/2)
\end{lstlisting}
\end{tabular}
\end{adjustbox}
\hspace{8pt}
% \vspace{10pt}
\begin{adjustbox}{valign=t,minipage=0.47\textwidth}
\begin{center}
    \underline{Fixed Program in Python}
\end{center} 
\begin{tabular}{l}
\lstset{escapechar=@,style=CustomPy}
\begin{lstlisting}[ 
    linebackgroundcolor={%
    \ifnum\value{lstnumber}=2
            \color{green!10}
    \fi
    }
]
n = int(input())
n = print(int((n-1+1)*(n-1)/2))
\end{lstlisting}

\end{tabular}
\end{adjustbox}
\end{tabular}
\vspace{6mm}

\begin{tabular}{p{13.5cm}}
\toprule
Model learned add sort function correctly \\
\bottomrule
\end{tabular}

\centering

\vspace{5pt}
\begin{tabular}{l}
\begin{adjustbox}{valign=t,minipage=0.47\textwidth}
\begin{center}
    \underline{Buggy Program in Python}
\end{center}
\begin{tabular}{l}

\lstset{escapechar=~,style=CustomPy}
\begin{lstlisting}[ 
    linebackgroundcolor={%
    \ifnum\value{lstnumber}=3
        \color{red!10}
    \fi
    }
]
n = int(input())
a = list(map(int,input().split())).sort()
print(a[-1]-a[0])

\end{lstlisting}
\end{tabular}
\end{adjustbox}
\hspace{8pt}
% \vspace{10pt}
\begin{adjustbox}{valign=t,minipage=0.47\textwidth}
\begin{center}
    \underline{Fixed Program in Python}
\end{center} 
\begin{tabular}{l}
\lstset{escapechar=@,style=CustomPy}
\begin{lstlisting}[ 
    linebackgroundcolor={%
    \ifnum\value{lstnumber}=3
            \color{green!10}
    \fi
    }
]
n = int(input())
a = list(map(int,input.split()))
a.sort()
print(a[-1]-a[0])

\end{lstlisting}
\end{tabular}
\end{adjustbox}
\end{tabular}

\vspace{6mm}

\begin{tabular}{p{13.5cm}}
\toprule
Model Learned to change the comparison sign \\
\bottomrule
\end{tabular}

\centering

\vspace{5pt}
\begin{tabular}{l}
\begin{adjustbox}{valign=t,minipage=0.47\textwidth}
\begin{center}
    \underline{Buggy Program in Python}
\end{center}
\begin{tabular}{l}

\lstset{escapechar=~,style=CustomPy}
\begin{lstlisting}[ 
    linebackgroundcolor={%
    \ifnum\value{lstnumber}=5
        \color{red!10}
    \fi
    }
]
N, K = map(int, input().split())
h = input().split()
c = 0
for i in range(N):
    if int(h[i]) > k:
        c += 1
print(c)
\end{lstlisting}
\end{tabular}
\end{adjustbox}
\hspace{8pt}
% \vspace{10pt}
\begin{adjustbox}{valign=t,minipage=0.47\textwidth}
\begin{center}
    \underline{Fixed Program in Python}
\end{center} 
\begin{tabular}{l}
\lstset{escapechar=@,style=CustomPy}
\begin{lstlisting}[ 
    linebackgroundcolor={%
    \ifnum\value{lstnumber}=5
            \color{green!10}
    \fi
    }
]
N, K = map(int, input().split())
h = input().split()
c = 0
for i in range(N):
    if int(h[i]) > k:
        c += 1
print(c)
\end{lstlisting}
\end{tabular}
\end{adjustbox}
\end{tabular}

\vspace{6mm}

\begin{tabular}{p{13.5cm}}
\toprule
Model Learned to change loop range for corrcetion\\
\bottomrule
\end{tabular}

\centering

\vspace{5pt}
\begin{tabular}{l}
\begin{adjustbox}{valign=t,minipage=0.47\textwidth}
\begin{center}
    \underline{Buggy Program in Python}
\end{center}
\begin{tabular}{l}

\lstset{escapechar=~,style=CustomPy}
\begin{lstlisting}[ 
    linebackgroundcolor={%
    \ifnum\value{lstnumber}=4
        \color{red!10}
    \fi
    }
]
from collections import defaultdict
N = int(input())
d = defaultdict(int)
for n in range(N):
    n = str(n)
    a = n[0]
    b = n[- 1]
    d[(a,b)] += 1
s = 0
for i in range(1, 10):
    for j in range(10):
        s += d[(str(j), str(i))] * d[(str(i), str(j))]
print(s)
\end{lstlisting}
\end{tabular}
\end{adjustbox}
\hspace{8pt}
% \vspace{10pt}
\begin{adjustbox}{valign=t,minipage=0.47\textwidth}
\begin{center}
    \underline{Fixed Program in Python}
\end{center} 
\begin{tabular}{l}
\lstset{escapechar=@,style=CustomPy}
\begin{lstlisting}[ 
    linebackgroundcolor={%
    \ifnum\value{lstnumber}=4
            \color{green!10}
    \fi
    }
]
from collections import defaultdict
N = int(input())
d = defaultdict(int)
for n in range(N+1):
    n = str(n)
    a = n[0]
    b = n[- 1]
    d[(a,b)]+=1
s = 0
for i in range(1,10):
    for j in range(10):
        s += d[(str(j), str(i))] * d[(str(i), str(j))]
print(s)
\end{lstlisting}
\end{tabular}
\end{adjustbox}
\end{tabular}

\caption{
Examples of successful fixes of buggy programs in Python. Buggy and fixed statements are marked in red and green, respectively.
}
\label{fig:example_2_python}
\end{figure*}

%\input{figure/python_generations}

% \newpage
% \subsection{Generated Java code examples with the CodeT5 model in Figure \ref{fig:examples_java}}
\begin{figure*}[t]
\centering

\vspace{5pt}

\begin{tabular}{p{13.5cm}}
\toprule
Model learned to copy entire line out of scope\\
\bottomrule
\end{tabular}
\begin{tabular}{l}
\begin{adjustbox}{valign=t,minipage=0.47\textwidth}
\begin{center}
    \underline{Buggy Program (Wrong Answer)}
\end{center}
\begin{tabular}{l}

\lstset{escapechar=~,style=CustomJava}
\begin{lstlisting}[ 
    linebackgroundcolor={%
    \ifnum\value{lstnumber}=11
        \color{red!10}
    \fi
    }
]
import java.util.*;
public class Main {
    public static void main(String[] args){
        Scanner sc = new Scanner(System.in);
        int D = sc.nextInt();
        int N = sc.nextInt();
        int a;
        a = (int) Math.pow(100, D )*N;
        if (N == 100){
            a = (int) Math.pow(100, D)*(N+1);
            System.out.println(a);
        }
    }
}
\end{lstlisting}
\end{tabular}
\end{adjustbox}
\hspace{8pt}
% \vspace{10pt}
\begin{adjustbox}{valign=t,minipage=0.47\textwidth}
\begin{center}
    \underline{Fixed Program}
\end{center} 
\begin{tabular}{l}
\lstset{escapechar=@,style=CustomJava}
\begin{lstlisting}[ 
    linebackgroundcolor={%
    \ifnum\value{lstnumber}=12
            \color{green!10}
    \fi
    }
]
import java.util.*;
public class Main {
    public static void main(String[] args){
        Scanner sc = new Scanner(System.in);
        int D = sc.nextInt();
        int N = sc.nextInt();
        int a;
        a = (int) Math.pow(100, D )*N;
        if (N == 100){
            a = (int) Math.pow(100, D)*(N+1);
        }
        System.out.println(a);
    }
}
\end{lstlisting}

\end{tabular}
\end{adjustbox}
\end{tabular}

\centering

\vspace{5pt}

\begin{tabular}{p{13.5cm}}
\toprule
Model learned change logic from "or" to "and" \\
\bottomrule
\end{tabular}
\begin{tabular}{l}
\begin{adjustbox}{valign=t,minipage=0.47\textwidth}
\begin{center}
    \underline{Buggy Program (Wrong Answer)}
\end{center}
\begin{tabular}{l}

\lstset{escapechar=~,style=CustomJava}
\begin{lstlisting}[ 
    linebackgroundcolor={%
    \ifnum\value{lstnumber}=7
        \color{red!10}
    \fi
    }
]
import java.util.*;
public class Main {
    public static void main(String[] args){
        Scanner sc = new Scanner(System.in);
        int a = sc.nextInt();
        int b = sc.nextInt();
        if ( a <= 8 || b <= 8 ) {
            System.out.println("Yay!");
        }
        else {
            System.out.println(":(");
        }
    }
}
\end{lstlisting}
\end{tabular}
\end{adjustbox}
\hspace{8pt}
% \vspace{10pt}
\begin{adjustbox}{valign=t,minipage=0.47\textwidth}
\begin{center}
    \underline{Fixed Program}
\end{center} 
\begin{tabular}{l}
\lstset{escapechar=@,style=CustomJava}
\begin{lstlisting}[ 
    linebackgroundcolor={%
    \ifnum\value{lstnumber}=7
            \color{green!10}
    \fi
    }
]
import java.util.*;
public class Main {
    public static void main(String[] args){
        Scanner sc = new Scanner(System.in);
        int a = sc.nextInt();
        int b = sc.nextInt();
        if ( a <= 8 && b <= 8 ) {
            System.out.println("Yay!");
        }
        else {
            System.out.println(":(");
        }
    }
}
\end{lstlisting}
\end{tabular}
\end{adjustbox}
\end{tabular}

\centering
\vspace{5pt}
\begin{tabular}{p{13.5cm}}
\toprule
Model Learned to change return statement to a print statement \\
\bottomrule
\end{tabular}
\begin{tabular}{l}
\begin{adjustbox}{valign=t,minipage=0.47\textwidth}
\begin{center}
    \underline{Buggy Program (Compilation Error)}
\end{center}
\begin{tabular}{l}

\lstset{escapechar=~,style=CustomJava}
\begin{lstlisting}[ 
    linebackgroundcolor={%
    \ifnum\value{lstnumber}=8
        \color{red!10}
    \fi
    }
]
import java.util.*;
public class Main {
    public static void main(String[] args){
        Scanner sc = new Scanner(System.in);
        int a = sc.nextInt();
        int a2 = a * a;
        int a3 = a2 * a;
        return a + a2 + a3;
    }
}
\end{lstlisting}
\end{tabular}
\end{adjustbox}
\hspace{8pt}
% \vspace{10pt}
\begin{adjustbox}{valign=t,minipage=0.47\textwidth}
\begin{center}
    \underline{Fixed Program}
\end{center} 
\begin{tabular}{l}
\lstset{escapechar=@,style=CustomJava}
\begin{lstlisting}[ 
    linebackgroundcolor={%
    \ifnum\value{lstnumber}=8
            \color{green!10}
    \fi
    }
]
import java.util.*;
public class Main {
    public static void main(String[] args){
        Scanner sc = new Scanner(System.in);
        int a = sc.nextInt();
        int a2 = a * a;
        int a3 = a2 * a;
        System.out.println( a + a2 + a3 );
    }
}
\end{lstlisting}
\end{tabular}
\end{adjustbox}
\end{tabular}

\centering
\vspace{5pt}
\begin{tabular}{p{13.5cm}}
\toprule
Model Learned to change syntax and compilation error \\
\bottomrule
\end{tabular}
\begin{tabular}{l}
\begin{adjustbox}{valign=t,minipage=0.47\textwidth}
\begin{center}
    \underline{Buggy Program (Compilation Error)}
\end{center}
\begin{tabular}{l}

\lstset{escapechar=~,style=CustomJava}
\begin{lstlisting}[ 
    linebackgroundcolor={%
    \ifnum\value{lstnumber}=8
        \color{red!10}
    \fi
    }
]
import java.util.*
public class Main {
    public static void main(String [] args){
        Scanner sc = new Scanner(System.in);
        int A = sc.nextInt();
        int B = sc.nextInt();
        int T = sc.nextInt();
        int S = T/A System.out.println(s*b);
    }
}
\end{lstlisting}
\end{tabular}
\end{adjustbox}
\hspace{8pt}
% \vspace{10pt}
\begin{adjustbox}{valign=t,minipage=0.47\textwidth}
\begin{center}
    \underline{Fixed Program}
\end{center} 
\begin{tabular}{l}
\lstset{escapechar=@,style=CustomJava}
\begin{lstlisting}[ 
    linebackgroundcolor={%
    \ifnum\value{lstnumber}=8
            \color{green!10}
    \fi
    \ifnum\value{lstnumber}=9
            \color{green!10}
    \fi
    }
]
import java.util.*
public class Main {
    public static void main(String [] args){
        Scanner sc = new Scanner(System.in);
        int A = sc.nextInt();
        int B = sc.nextInt();
        int T = sc.nextInt();
        int S = T/A;
        System.out.println(s*B);
    }
}
\end{lstlisting}
\end{tabular}
\end{adjustbox}
\end{tabular}

\caption{
Examples of successful fixes of buggy programs in Java. Buggy and fixed statements are marked in red and green, respectively.
}
\label{fig:examples_java}
\end{figure*}
